# Supplementary material for: ViGoR: Improving Visual Grounding of Large Vision Language Models with Fine-Grained Reward Modeling
Source: arXiv:2402.06118 source file (2025-12-22)
Supplement: Supplementary file 1 [file supp.tex]

In this document, we provide further details about our work, focusing on the data gathering and usage of our reward model, performance evaluation setup, and metrics. Finally, we present additional qualitative results to provide more anecdotal insight into the effectiveness of our model.

\section{Visual Grounding Improvement Framework Details}

\subsection{Details of Reward Modeling via Fine-Grained Human Feedback}

\subsubsection{Human Annotation} 
\label{sec:human}
In this section, we give some clarifying details about our human annotation framework for collecting preference feedback. 

\paragraph{Data source:} To collect human annotation, we first select a group of images and sample a set of responses by the LVLM. In our case, we sample 7,200 images from the \textit{train2017} split from the MS COCO dataset. Because of the expense of collecting human annotations, it is desirable for the reward model to learn more fine-grained and holistic signals that will allow it to further improve a relatively strong initial starting point of the LVLM. As shown in our main article, our automated signal generation approach can already significantly improve the visual grounding of the LLaVA model. Therefore, we generate responses using the checkpoint fine-tuned using only the automatic supervision approach. In particular, we generate 15,440 responses using the following prompts. 

\begin{itemize}
\item   Describe the given image in detail.
\item  Write a detailed description of the given image.
\item  Give a detailed description of the given image.
\item  Explain the visual content of the image in great detail.
\item  Analyze the image in a comprehensive and detailed manner.
\end{itemize}

\paragraph{Annotation Instructions:} For each image-description pair, we ask annotators to carefully consider each sentence of the description in two aspects: \textit{accuracy} and \textit{creativity}. \textit{Accuracy} refers to whether the sentence is factually correct. The annotator is asked to select one of the following categories for each sentence. 

\begin{itemize}
    \item Accurate - all details mentioned in this sentence are true with respect to the input image. 
    \item Hallucinated object - the sentence mentions an object that does not exist in the image. 
    \item Incorrect object color - the sentence describes an object that exists in the image with the wrong color. 
    \item Incorrect object quantity - the sentence describes an object that exists in the image with the wrong count. 
    \item Incorrect object material - the sentence describes an object that exists in the image to be made of the wrong material. 
    \item Incorrect object shape - the sentence describes an object that exists in the image to be the wrong shape. 
    %\item Incorrect object (other) - the sentence assigns wrong descriptions to an object in the image in a different way than the above. 
    \item Incorrect object relationship - the sentence describes the relationship between two or more objects incorrectly. For example, the sentence mentions that \textit{a person is riding a bicycle}, while the person is actually pushing the bicycle in the image. 
    \item Incorrect object location - the sentence mentions objects with the wrong localization in the image. 
    \item Incorrect reasoning: the sentence describes an illogical interpretation of the image. For example, the image shows an empty and dilapidated street, but the text describes it to be \textit{lively and cheerful}. 
    \item Other - the sentence assigns wrong descriptions in the image in a different way than the above. 

\end{itemize}

Furthermore, the \textit{creativity} score is a binary assessment of whether the sentence attempts to provide a reasonable interpretation of the extrapolation of the image. For example, a sentence such as \textit{``The potted plants contribute to a pleasant and calming atmosphere in the room.} is considered creative, while \textit{ ``There is a potted plant on the table."} is not. 

Lastly, we ask annotators to perform a holistic assessment of the overall description's \textit{level of detail} (as a score between 1 and 7) with the following rubric. 

{\itshape \small
Ignore the accuracy, how comprehensively does the description capture the image's key elements?

\begin{itemize}
    \item 1 = Extremely Lacking: The description omits all vital information.
    \item 2 = Lacking: The description only has a summary without any description of the objects.
    \item 3 = Somewhat Lacking: The description only has a summary but misses most detailed description of the objects in the image.
    \item 4 = Neutral: The description only contains the details of few objects in the image.
    \item 5 = Somewhat detailed: The description contains the details of most of the objects but misses two or three key elements in the image.
    \item 6 = Detailed: The description covers nearly all the objects but misses one key element in the image.
    \item 7 = Extremely Detailed: The description covers all essential details present in the image.
\end{itemize}
}

%Finally, we ask the annotator to note the \textit{major} objects in the scene missed by the description. 

\begin{algorithm}
\caption{Human Feedback Reward Model Score}
\begin{algorithmic}[1]

\footnotesize

\State \textbf{Input:} $Image$, \{\textit{Descriptions}\}, Trained Reward Model $R_H$
    \For{each $S_i$ in \{\textit{Descriptions}\}}
        \State Divide $S_i$ into a set of sentences $\{s_{i,1}, s_{i,2}, \ldots, s_{i,m}\}$
        \State $P^h_i \gets 0$
        \State $N^h_i \gets 0$
        \For{each sentence $s_{i,j}$ in $\{s_{i,1}, s_{i,2}, \ldots, s_{i,m}\}$}
            \If{$R_H(s_{i,j}, \{s_{i,1}, s_{i,2}, \ldots, s_{i,j-1}\}, Image)$ = 0}
                \State $P^h_i \gets P^h_i + 1$
            \Else
                \State $N^h_i \gets N^h_i + 1$
            \EndIf
        \EndFor
        \State The final scores for $S_i$ are $(N^h_i, P^h_i)$
    \EndFor
\end{algorithmic}
\label{alg:human}
\end{algorithm}

\subsubsection{Reward Model Training} % Siming
After collecting human annotation data, we proceed to train a reward model. In our implementation, we adopt the same architecture as the LLaVA model for the reward model. We initialize the weights of the reward model using the pre-trained LLaVA model and then fine-tune it using the human annotation data. As mentioned in Section~\ref{sec:human}, our reward model predicts the \textit{accuracy} score, which is a discrete integer ranging from 0 to 9, with the following categories: 0: Accurate, 1: Hallucinated object, 2: Incorrect object color, 3: Incorrect object quantity, 4: Incorrect object material, 5: Incorrect object shape, 6: Incorrect object relationship, 7: Incorrect object location, 8: Incorrect reasoning, 9: Others. %The creativity score is represented as a binary integer, where 1 and 0 correspond to a sentence which does and does not attempt to make any creative assessments of the sentence, respectively.

Inspired by~\cite{chen2021pix2seq}, unlike the traditional approach of adding a linear layer for direct score regression, we treat the task as a language modeling problem, leveraging the inherent capabilities of the reward model. We observe that it has shown enhanced stability compared to direct score regression. To effectively gauge the accuracy, we have designed a specific prompt. It guides the reward model to evaluate the last sentence in a given image description, assigning a numerical value based on various criteria.

{\itshape \small
Assess the accuracy of the last sentence in the following description of this image and return a single number: 0 for accurate, 1 for hallucination of objects, 2 for incorrect object color, 3 for incorrect number of objects, 4 for incorrect object material, 5 for incorrect object shape, 6 for incorrect object relationship, 7 for incorrect object location, 8 for flawed reasoning and 9 for other types of inaccuracies. 

\noindent Description: ...
}

% Similarly, for the creativity score, the prompt has been tailored to assess the last sentence of the image description. Creativity is rated on a binary scale from 0 (non-creative) to 1 (creative), allowing for a straightforward yet effective evaluation of the creative aspect:

% {\itshape \small
% Assess the creativity score of the last sentence in the following description of this image. Rate the creativity on a scale from 0 to 1, where 0 represents non-creative and 1 represents creative.

% \noindent Description: ...
% }

The model is trained to predict the numerical score in text format. This method not only streamlines the evaluation process but also aligns with the intrinsic strengths of the language model, facilitating more nuanced and stable scoring.

In practice, we find that the \textit{creativity}, \textit{level of detail} and \textit{missing objects} judgment for the holistic description by our annotators is unfortunately somewhat difficult to combine into our rejection sampling scheme. Therefore, we opted to ignore these annotated attributes in the models presented. However, we believe that they will be beneficial for future work.

\subsubsection{Reward Model Scoring}

Upon completing the training of the reward model, it is employed to assign rewards to each description generated by LVLM. As the model provides sentence-level scores, these must be consolidated to derive an overall score for each description. To this end, we compute two distinct scores for each description: a positive score, denoted as $P^h$, and a negative score, denoted as $N^h$. The scoring process is as follows: for each sentence that the reward model evaluates as accurate (returning a value of 0), the positive score $P^h$ is incremented by 1. Conversely, for each sentence deemed inaccurate, the negative score $N^h$ is incremented by 1. This scoring method is elaborated upon in Algorithm~\ref{alg:human}.

\begin{figure}[t]
    \centering
    \includegraphics[width=0.8\linewidth]{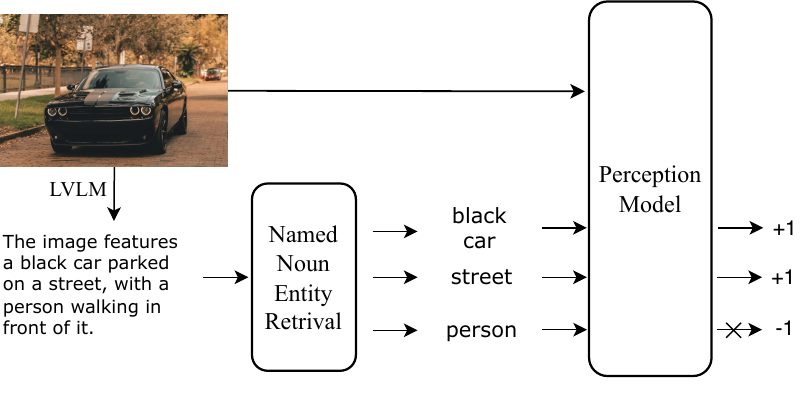}
    \caption{\textbf{Illustration of reward modeling with automatic methods.}}
    \label{fig:automatic_model}
\end{figure}

\subsection{Details of Reward Modeling with Automatic Methods}

In this section, we show more details on the implementation of reward modeling with automatic methods. As shown in Figure~\ref{fig:automatic_model}, given a description generated by LVLM from an image, we first identify the individual nouns mentioned using standard recognition of the entity of nouns. 

Following the identification of noun phrases, each is paired with the original image and analyzed using a perception model. In our implementation, we employ an open-set detector, Grounding DINO~\cite{liu2023grounding}, for this purpose. The core function of this model is to verify the presence of the identified noun phrases within the image. 

Similar to the approach of reward modeling that leverages detailed human feedback, the scoring process of the reward model for automatic methods also yields two distinct scores for each description: a positive score $P^a$ and a negative score $N^a$. A positive score (+1) is assigned if the noun phrase is successfully detected in the image, for example, `black car' and `street' in this case. Conversely, if the perception model fails to locate the noun phrase in the image (e.g., `person'), a negative score (-1) is attributed. This scoring method is elaborated upon in Algorithm~\ref{alg:auto}.

\begin{algorithm}[t]
\caption{Automatic Method Reward Model Score}
\begin{algorithmic}[1]
\State \textbf{Input:} $Image$, \{\textit{Descriptions}\}, Perception Model $R_A$
    \For{each $S_i$ in \{\textit{Descriptions}\}}
        % \State Divide $S_i$ into a set of sentences $\{s_{i,1}, s_{i,2}, \ldots, s_{i,m}\}$
        \State $P^a_i \gets 0$
        \State $N^a_i \gets 0$
        \For{each noun phrase $n_{i,j}$ in $S_i$}
            \If{$n_{i,j}$ is detected by $R_A$}
                \State $P_i^a \gets P^a_i + 1$
            \Else
                \State $N_i^a \gets N^a_i + 1$
            \EndIf
        \EndFor
        \State The final scores for $S_i$ are $(N^a_i, P^a_i)$
    \EndFor
\end{algorithmic}
\label{alg:auto}
\end{algorithm}

% \State \textbf{Input:} $Image$, \{\textit{Descriptions}\}, Trained Reward Model $R_H$
%     \For{each $S_i$ in \{\textit{Descriptions}\}}
%         \State Divide $S_i$ into a set of sentences $\{s_{i,1}, s_{i,2}, \ldots, s_{i,m}\}$
%         \State $P^h_i \gets 0$
%         \State $N^h_i \gets 0$
%         \For{each sentence $s_{i,j}$ in $\{s_{i,1}, s_{i,2}, \ldots, s_{i,m}\}$}
%             \If{$R_H(s_{i,j}, \{s_{i,1}, s_{i,2}, \ldots, s_{i,j-1}\}, Image)$ = 0}
%                 \State $P^h_i \gets P^h_i + 1$
%             \Else
%                 \State $N^h_i \gets N^h_i + 1$
%             \EndIf
%         \EndFor
%         \State The final scores for $S_i$ are $(N^h_i, P^h_i)$
%     \EndFor

\subsection{Details of Reward Score Combination and Rejection Sampling}

In this section, we provide a detailed exposition and clarification of the process for combining reward scores, as well as the subsequent rejection sampling procedure. 

\subsubsection{Reward Score Combination}
For each description, we obtain fine-grained reward scores from two sources: reward modeling via detailed human feedback and automated methods, denoted as $(N^h, P^h)$ and $(N^a, P^a)$, respectively. To compute the final score for each description, we sum the negative and positive scores separately, resulting in a composite score: $(N, P) = (N^h + N^a, P^h + P^a)$. 

\subsubsection{Rejection Sampling Procedure}

A general procedure of rejection sampling for LVLM is depicted in Figure~\ref{fig:rejection}. The process begins with the generation of $N$ samples from LVLM. Each of these samples is evaluated by the reward modeling module, which assigns a specific reward score to each sample. The rejection sampling module selects the best sample according to the reward score.

In our case, the best sample is the one with the smallest $N$. If there are multiple descriptions with the same smallest $N$, then the one with the largest $P$ is chosen as a tiebreaker. This best sample is used as the regression target in the supervised fine-tuning setting to improve the LVLM. 

\begin{figure}
    \centering
    \includegraphics[width=0.8\linewidth]{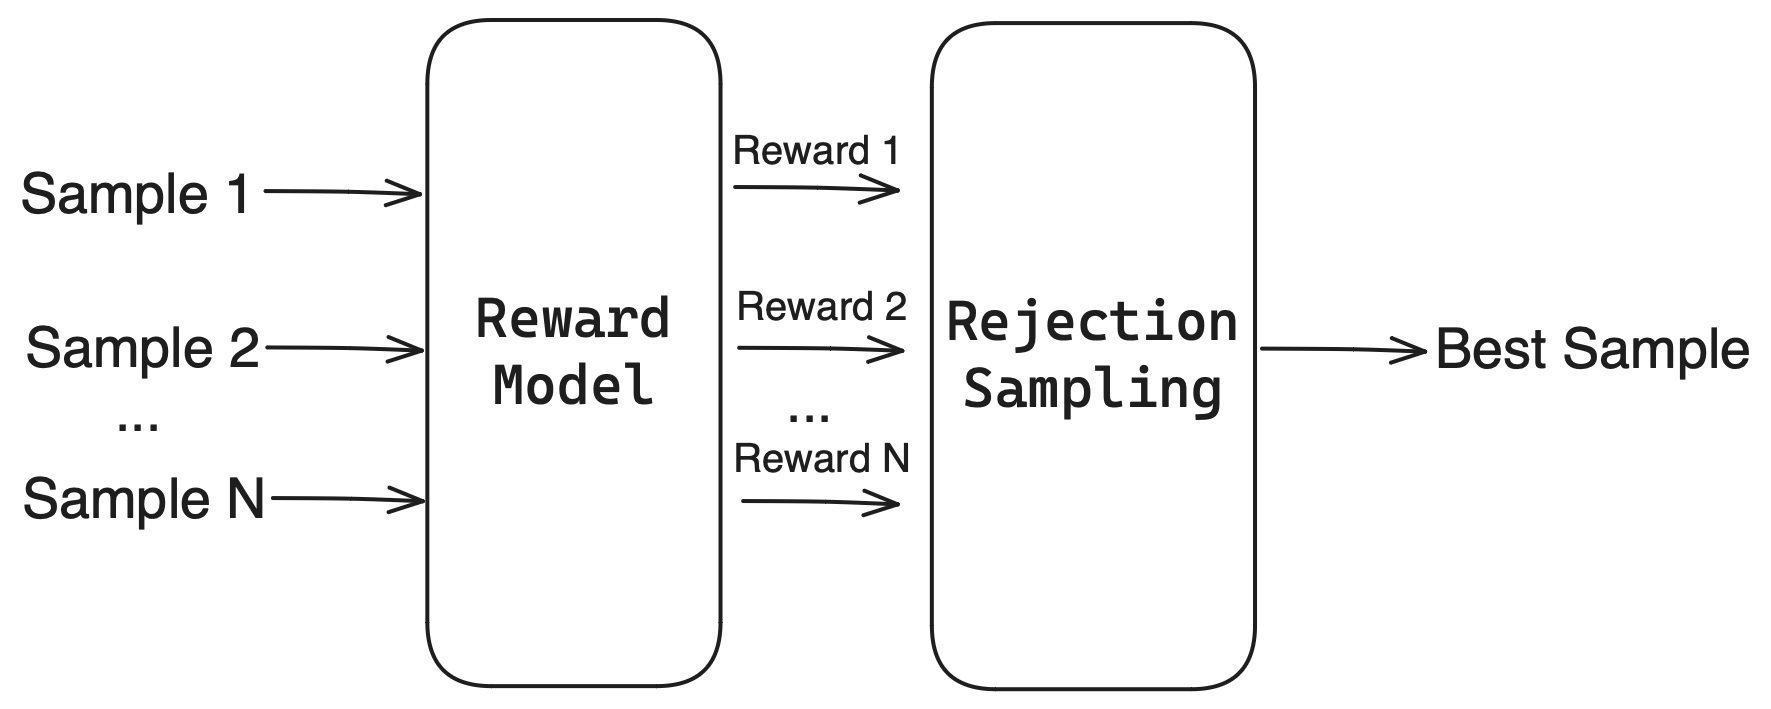}
    \caption{\textbf{Illustration of the rejection sampling procedure.}}
    \label{fig:rejection}
\end{figure}

\subsection{Details of Refinement Module}
In this section, we provide a detailed overview of the refinement module. 
%This module plays a crucial role in processing descriptions obtained from the rejection sampling module. 
The core of our strategy lies in a straightforward refinement approach applied to the sample descriptions.

For each sentence within the description, we assess the presence of noun phrases deemed nonexistent by the reward modeling module. Should a sentence contain any such noun phrases, we eliminate that sentence entirely from the description. For instance, consider the description:\textit{``The image features a black Dodge Charger parked on a brick road next to a sidewalk. A person is walking in front of the car."} If the reward modeling module identifies \textit{`person'} as a non-existent noun phrase, the sentence \textit{``A person is walking in front of the car."} is removed.

This refinement process effectively reduces the hallucination problem by removing inaccurate elements, thereby leading to notable improvements in the model's performance.

\section{Performance Evaluation Details}

\subsection{Detailed Description Generation Evaluation} 

Objective and consistent evaluation of free-form text output has traditionally been a difficult problem. Previously, the research community has often relied on handcrafted metrics such as BLEU \cite{papineni-etal-2002-bleu} and ROUGE \cite{lin-2004-rouge} to evaluate the similarity between text. However, these generally only reward regurgitation of the exact same passage as the ground truth, but disregard high-level meaning and alternative but equally valid expression. We elect to use the powerful proprietary GPT-4Vision (with impressive prompt follow-up and visual recognition capabilities \cite{yang2023dawn}) as a tool to give us an imperfect yet still valuable method to evaluate the descriptions generated by various settings of our LVLM. 

As our task is fundamentally to compare the quality of generated results of different model settings, we select a set of images and generate a group of descriptions using each model setting to be compared. We then provide a single instruction to GPT-4Vision using the following template along with the underlying image. 
\begin{figure*}
    \centering
    \includegraphics[width=\linewidth]{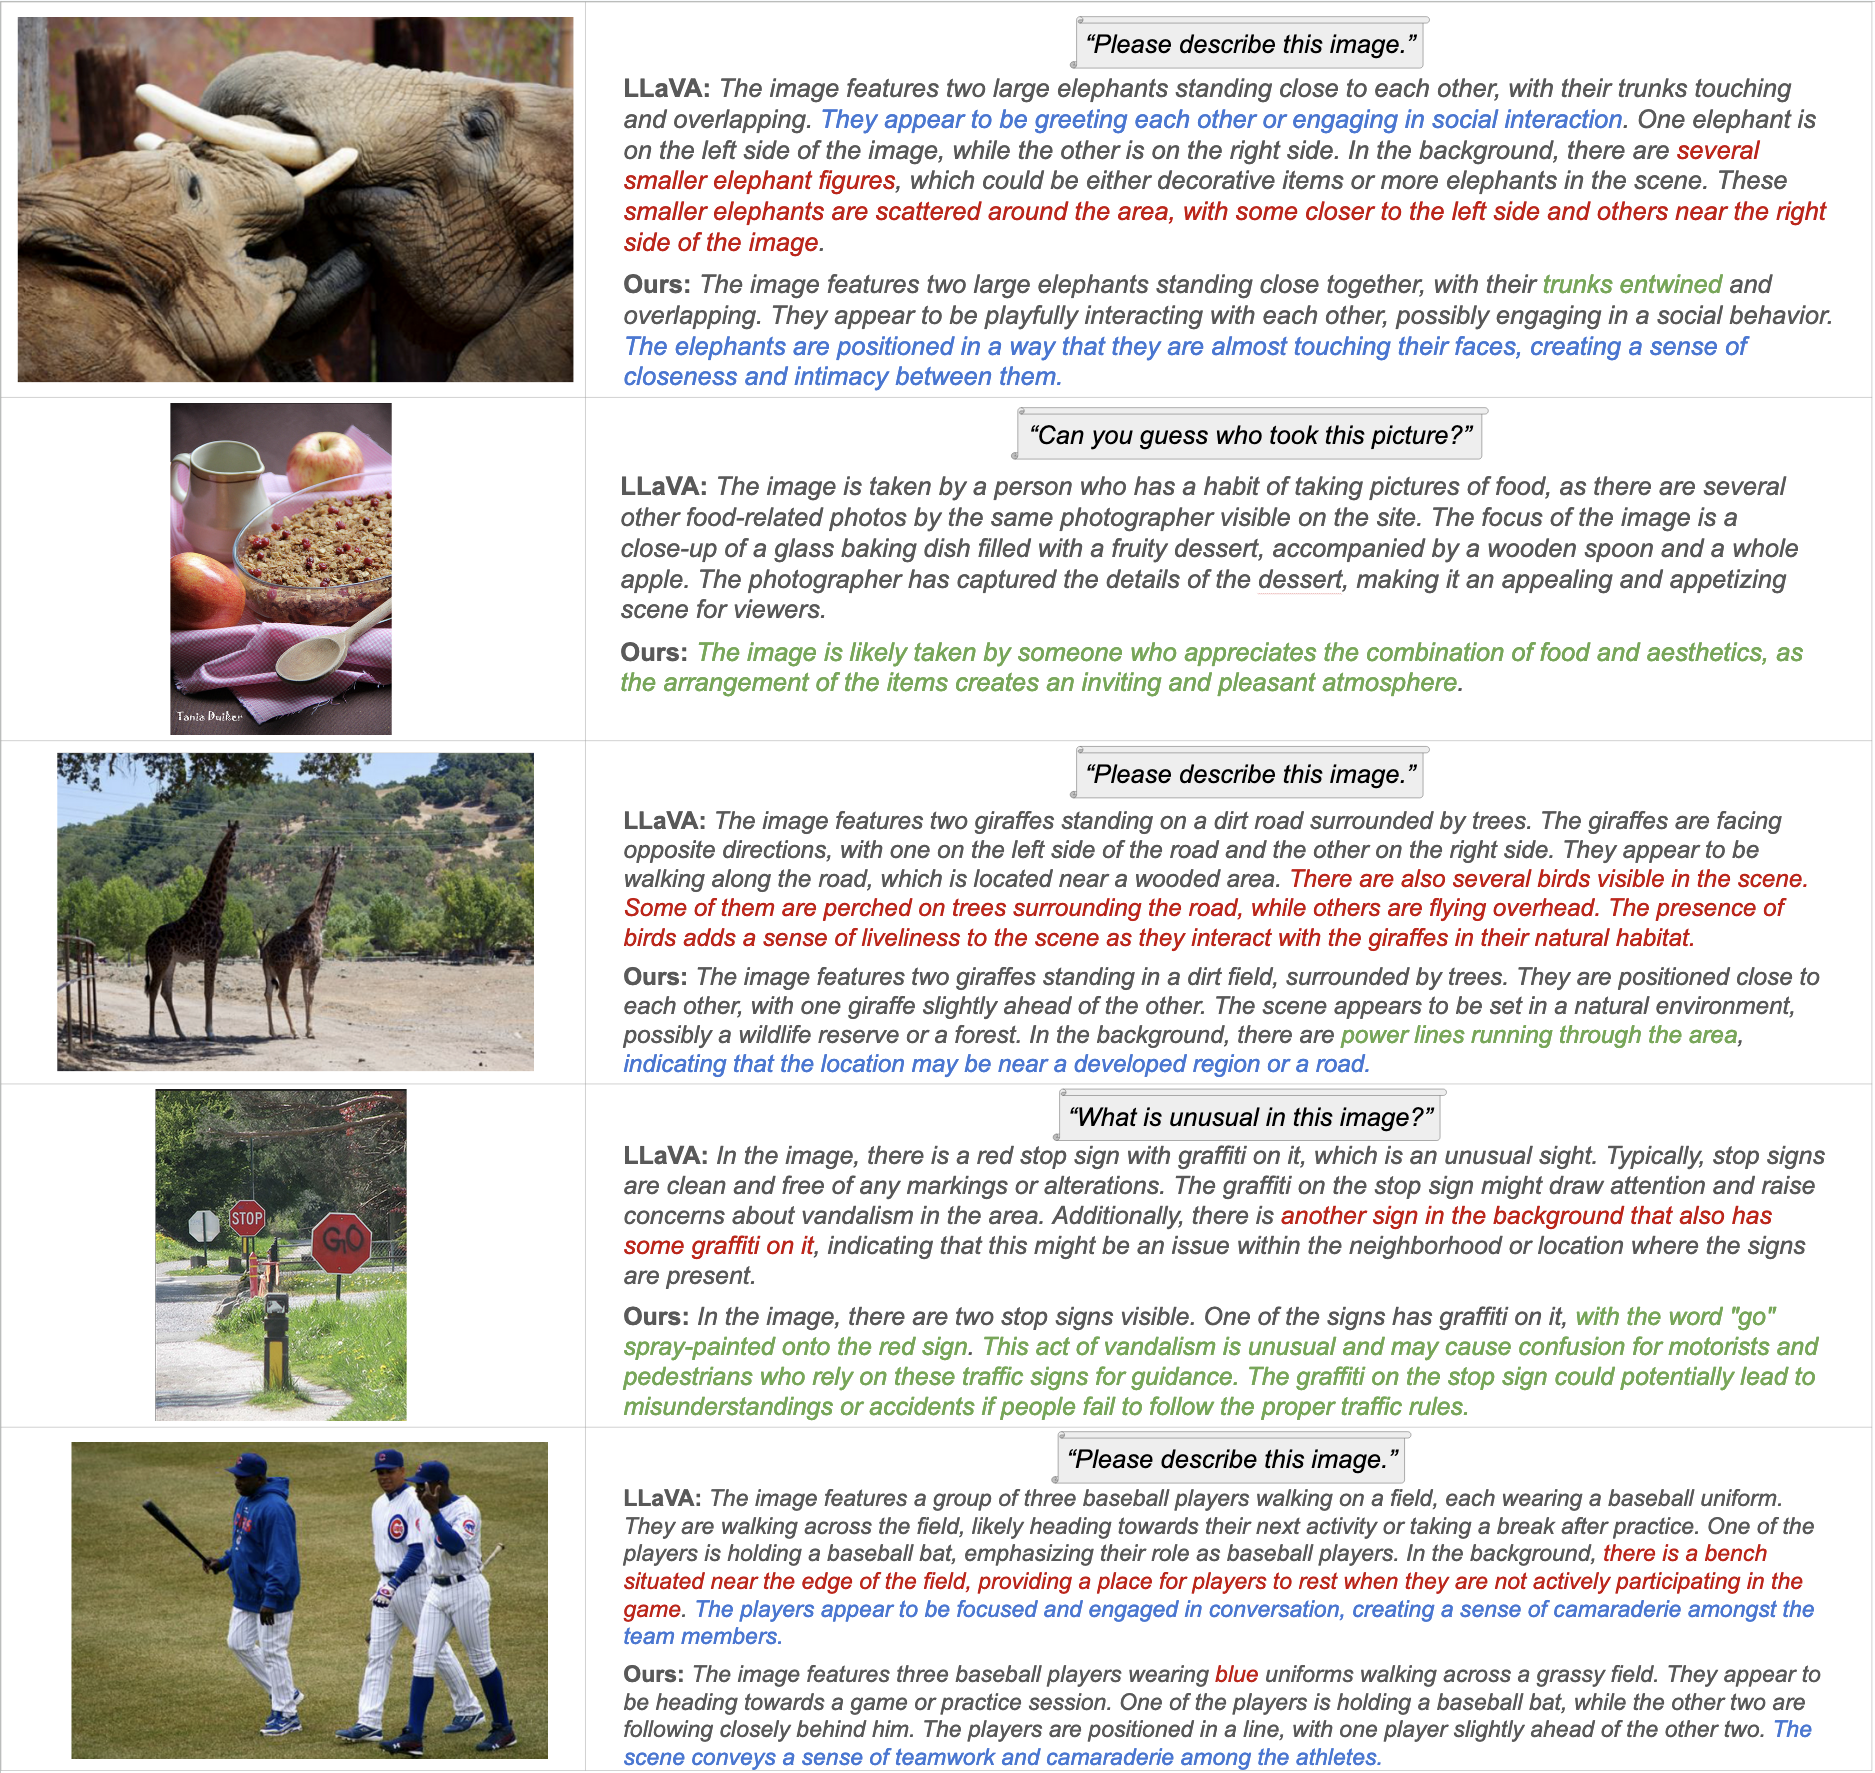}
    \caption{\textbf{Additional qualitative results.} We show examples of descriptions generated by our technique after using the fine-tuning scheme, and compare them with the output from the original LLaVA \cite{liu2023llava}. Our approach is able to greatly reduce the amount of \textcolor{brightmaroon}{hallucinations and invalid observations} while increasing the amount of \textcolor{dartmouthgreen}{detailed visual descriptions}. Furthermore, the model retains the \textcolor{denim}{plausible intuitive reasoning} capabilities of the underlying LLM. Please see Sec. \ref{qual_discussion} for further discussions. }
    \label{fig:qualitative_supp}
\end{figure*}
{\itshape \small

Please rank the following four descriptions of the provided image according to the following criteria.

Existence accuracy (EA): Evaluate whether the objects mentioned in the description exist in the image.

Counting accuracy (CA): Assess the accuracy in the number of objects described.

Accuracy of attributes (AA): Gauge the accuracy of the attributes (color, material, shape, etc.) assigned to the objects in the description.

Relation accuracy (RA): Consider how accurately the description captures the spatial or relational aspects of objects in the image (e.g., an object being on top of, next to, or inside another object).

Relevance (RL): Assess whether the description is relevant and relevant to the content of the image.

Reasoning (RS): Evaluate the description for reasonable interpretations or extrapolations about the image (e.g., 1. The general atmosphere of the bathroom appears to be in the process of being renovated or updated. 2. The overall atmosphere of the kitchen appears warm and welcoming. 3. It indicates that they are enjoying the time.)

Detail Level (DL): Measure the level of detail provided in the entire description, considering both the quantity and the quality of the details.

After completing the ranking, please use the following template to report your results, where the first item represents the best and the last the worst.

For example: EA: [0,2,3,1]; CA: [1,3,2,0]; AA: [3,2,1,0]; RA: [1,0,2,3]; RL: [0,3,2,1]; RS: [3,1,0,2], DL: [1,3,0,2]. DO NOT return any explanation. \\

\noindent Description 1: ... \\
Description 2: ... \\
Description 3: ... \\
Description 4: ... 

}

Upon retrieving the responses from GPT-4Vision, we aggregate the ranking information for each image's description set by computing the average rank within each metric type across the image samples. As such, the best average rank that a model can achieve within a particular metric is 1.0, while the worst is equal to the total number of competitor models, which is 4.0 in the above case. 

% \subsection{MMViG Benchmark Details} % Siming
% In our research, we identified a gap in the existing benchmarking systems for LVLM, particularly concerning the assessment of visual grounding capabilities. To address this, we have developed a new benchmark, MMViG (Multimodal Visual Grounding), designed to comprehensively evaluate the visual grounding ability of LVLMs.

% MMViG categorizes the assessment into four specific areas: Hallucinations (HL), Counting Accuracy (CA), Color Accuracy (CO), and Material Accuracy (MA). Our evaluation methodology involves the careful selection of 200 images from the MS COCO 2017 validation dataset for each category. Each image is paired with two questions. The structured question set is shown in Fig.~\ref{fig:mmvig}.

% The questions are formulated automatically using the annotations provided in the COCO and PACO datasets. This approach ensures that the questions are relevant, precise, and effectively tailored to test the specific aspects of visual grounding in LVLM. The MMViG benchmark, with its focused categories and methodical evaluation process, provides a more robust and comprehensive tool for assessing the visual grounding performance of LVLMs.

%\section{Further Ablation Studies} % Siming

\section{Additional Qualitative Results} \label{qual_discussion} % Min
In Figure~\ref{fig:qualitative_supp}, we provide additional samples of conversations that contrast the behavior of the LVLM before and after the fine-tuning using ViGoR. Through these varied examples, it is evident that our fine-tuning scheme focusing on improving visual grounding in creating detailed descriptions has strong generalization capability to other types of queries. In the first, third, and last rows, we see further cases in which our approach is able to produce more accurate descriptions with fewer incidents of hallucinations that are present in the responses of the original model. The second and fourth rows demonstrate that our approach is able to maintain the powerful abstract reasoning capabilities of the original LLM, but further refine its attention and visual grounding capacities. 

\section{Potential Negative Societal Impact}

In our experiments, we train and debug ViGoR using eight 40G A100 GPUs for approximately 100 hours.
The total emission is estimated to be 60.00 kgCO2eq, equivalent to 242.6 km driven by an average car. This estimation is conducted using the Machine Learning Impact calculator presented in~\cite{lacoste2019quantifying}. 

% To mitigate repetitive labor and negative environmental impact in future research, we plan to release our open-source implementation together with trained network weights.
